# Supplementary material for: Tighter Variational Bounds are Not Necessarily Better
Source: arXiv:1802.04537 source file (2019-03-05)
Supplement: Supplementary file 1 [file appendix.pdf]

---

# Tighter Variational Bounds are Not Necessarily Better

---

Tom Rainforth<sup>1</sup> Adam R. Kosiorek<sup>1,2</sup> Tuan Anh Le<sup>2</sup> Chris J. Maddison<sup>1</sup> Maximilian Igl<sup>2</sup> Frank Wood<sup>3</sup>  
Yee Whye Teh<sup>1</sup>

## Abstract

We provide theoretical and empirical evidence that using tighter evidence lower bounds (ELBOs) can be detrimental to the process of learning an inference network by reducing the signal-to-noise ratio of the gradient estimator. Our results call into question common implicit assumptions that tighter ELBOs are better variational objectives for simultaneous model learning and inference amortization schemes. Based on our insights, we introduce three new algorithms: the partially importance weighted auto-encoder (PIWAE), the multiply importance weighted auto-encoder (MIWAE), and the combination importance weighted auto-encoder (CIWAE), each of which includes the standard importance weighted auto-encoder (IWAE) as a special case. We show that each can deliver improvements over IWAE, even when performance is measured by the IWAE target itself. Furthermore, our results suggest that PIWAE may be able to deliver simultaneous improvements in the training of both the inference and generative networks.

---

<sup>1</sup>Department of Statistics, University of Oxford <sup>2</sup>Department of Engineering, University of Oxford <sup>3</sup>Department of Computer Science, University of British Columbia. Correspondence to: Tom Rainforth <rainforth@stats.ox.ac.uk>.

## Acknowledgments

TR and YWT are supported in part by the European Research Council under the European Union's Seventh Framework Programme (FP7/2007–2013) / ERC grant agreement no. 617071. TAL is supported by a Google studentship, project code DF6700. MI is supported by the UK EPSRC CDT in Autonomous Intelligent Machines and Systems. CJM is funded by a DeepMind Scholarship. FW is supported under DARPA PPAML through the U.S. AFRL under Cooperative Agreement FA8750-14-2-0006, Sub Award number 61160290-111668.

---

## Appendices for Tighter Variational Bounds are Not Necessarily Better

---

Tom Rainforth   Adam R. Kosiorek   Tuan Anh Le   Chris J. Maddison  
Maximilian Igl   Frank Wood   Yee Whye Teh

### A Proof of SNR Convergence Rates

**Theorem 1.** Assume that when  $M = K = 1$ , the expected gradients; the variances of the gradients; and the first four moments of  $w_{1,1}$ ,  $\nabla_{\theta} w_{1,1}$ , and  $\nabla_{\phi} w_{1,1}$  are all finite and the variances are also non-zero. Then the signal-to-noise ratios of the gradient estimates converge at the following rates

$$\text{SNR}_{M,K}(\theta) = \sqrt{M} \left| \frac{\sqrt{K} \nabla_{\theta} Z - \frac{1}{2Z\sqrt{K}} \nabla_{\theta} \left( \frac{\text{Var}[w_{1,1}]}{Z^2} \right) + O\left(\frac{1}{K^{3/2}}\right)}{\sqrt{\mathbb{E} \left[ w_{1,1}^2 (\nabla_{\theta} \log w_{1,1} - \nabla_{\theta} \log Z)^2 \right] + O\left(\frac{1}{K}\right)}} \right| \quad (\text{A.1})$$

$$\text{SNR}_{M,K}(\phi) = \sqrt{M} \left| \frac{\nabla_{\phi} \text{Var}[w_{1,1}] + O\left(\frac{1}{K}\right)}{2Z\sqrt{K} \sigma[\nabla_{\phi} w_{1,1}] + O\left(\frac{1}{\sqrt{K}}\right)} \right| \quad (\text{A.2})$$

where  $Z := p_{\theta}(x)$  is the true marginal likelihood.

*Proof.* We start by considering the variance of the estimators. We will first exploit the fact that each  $\hat{Z}_{m,K}$  is independent and identically distributed and then apply Taylor's theorem<sup>1</sup> to  $\log \hat{Z}_{m,K}$  about  $Z$ , using  $R_1(\cdot)$  to indicate the remainder term, as follows.

$$\begin{aligned} M \cdot \text{Var}[\Delta_{M,K}] &= \text{Var}[\Delta_{1,K}] = \text{Var} \left[ \nabla_{\theta, \phi} \left( \log Z + \frac{\hat{Z}_{1,K} - Z}{Z} + R_1(\hat{Z}_{1,K}) \right) \right] \\ &= \text{Var} \left[ \nabla_{\theta, \phi} \left( \frac{\hat{Z}_{1,K} - Z}{Z} + R_1(\hat{Z}_{1,K}) \right) \right] \\ &= \mathbb{E} \left[ \left( \nabla_{\theta, \phi} \left( \frac{\hat{Z}_{1,K} - Z}{Z} + R_1(\hat{Z}_{1,K}) \right) \right)^2 \right] - \left( \mathbb{E} \left[ \nabla_{\theta, \phi} \left( \frac{\hat{Z}_{1,K} - Z}{Z} + R_1(\hat{Z}_{1,K}) \right) \right] \right)^2 \\ &= \mathbb{E} \left[ \left( \frac{1}{K} \sum_{k=1}^K \frac{Z \nabla_{\theta, \phi} w_{1,k} - w_{1,k} \nabla_{\theta, \phi} Z}{Z^2} + \nabla_{\theta, \phi} R_1(\hat{Z}_{1,K}) \right)^2 \right] - \left( \cancel{\nabla_{\theta, \phi} \mathbb{E} \left[ \frac{\hat{Z}_{1,K} - Z}{Z} \right]} + \mathbb{E} \left[ \nabla_{\theta, \phi} R_1(\hat{Z}_{1,K}) \right] \right)^2 \\ &= \frac{1}{KZ^4} \mathbb{E} \left[ (Z \nabla_{\theta, \phi} w_{1,1} - w_{1,1} \nabla_{\theta, \phi} Z)^2 \right] + \text{Var} \left[ \nabla_{\theta, \phi} R_1(\hat{Z}_{1,K}) \right] \\ &\quad + 2 \mathbb{E} \left[ \left( \nabla_{\theta, \phi} R_1(\hat{Z}_{1,K}) \right) \left( \frac{1}{K} \sum_{k=1}^K \frac{Z \nabla_{\theta, \phi} w_{1,k} - w_{1,k} \nabla_{\theta, \phi} Z}{Z^2} \right) \right] \end{aligned}$$

Now we have by the mean-value form of the remainder that for some  $\tilde{Z}$  between  $Z$  and  $\hat{Z}_{1,K}$

$$R_1(\hat{Z}_{1,K}) = -\frac{(\hat{Z}_{1,K} - Z)^2}{2\tilde{Z}^2}$$

---

<sup>1</sup>This approach follows similar lines to the derivation of nested Monte Carlo convergence bounds in (Rainforth, 2017; Rainforth et al., 2018; Fort et al., 2017) and the derivation of the mean squared error for self-normalized importance sampling, see e.g. (Hesterberg, 1988).

and therefore

$$\nabla_{\theta,\phi} R_1(\hat{Z}_{1,K}) = -\frac{\tilde{Z}(\hat{Z}_{1,K} - Z) \nabla_{\theta,\phi}(\hat{Z}_{1,K} - Z) - (\hat{Z}_{1,K} - Z)^2 \nabla_{\theta,\phi} \tilde{Z}}{\tilde{Z}^3}.$$

It follows that the  $\nabla_{\theta,\phi} R_1(\hat{Z}_{1,K})$  terms are dominated as each of  $(\hat{Z}_{1,K} - Z) \nabla_{\theta,\phi}(\hat{Z}_{1,K} - Z)$  and  $(\hat{Z}_{1,K} - Z)^2$  vary with the square of the estimator error, whereas other comparable terms vary only with the unsquared difference. The assumptions on moments of the weights and their derivatives further guarantee that these terms are finite. More precisely, we have  $\tilde{Z} = Z + \alpha(\hat{Z}_{1,K} - Z)$  for some  $0 < \alpha < 1$  where  $\nabla_{\theta,\phi} \alpha$  must be bounded with probability 1 as  $K \rightarrow \infty$  to maintain our assumptions. It follows that  $\nabla_{\theta,\phi} R_1(\hat{Z}_{1,K}) = O((\hat{Z}_{1,K} - Z)^2)$  and thus that

$$\text{Var}[\Delta_{M,K}] = \frac{1}{MKZ^4} \mathbb{E}[(Z \nabla_{\theta,\phi} w_{1,1} - w_{1,1} \nabla_{\theta,\phi} Z)^2] + \frac{1}{M} O\left(\frac{1}{K^2}\right) \quad (\text{A.3})$$

using the fact that the third and fourth order moments of a Monte Carlo estimator both decrease at a rate  $O(1/K^2)$ .

Considering now the expected gradient estimate and again using Taylor's theorem, this time to a higher number of terms,

$$\begin{aligned} \mathbb{E}[\Delta_{M,K}] &= \mathbb{E}[\Delta_{1,K}] = \mathbb{E}[\Delta_{1,K} - \nabla_{\theta,\phi} \log Z] + \nabla_{\theta,\phi} \log Z \\ &= \nabla_{\theta,\phi} \mathbb{E} \left[ \log Z + \frac{\hat{Z}_{1,K} - Z}{Z} - \frac{(\hat{Z}_{1,K} - Z)^2}{2Z^2} + R_2(\hat{Z}_{1,K}) - \log Z \right] + \nabla_{\theta,\phi} \log Z \\ &= -\frac{1}{2} \nabla_{\theta,\phi} \mathbb{E} \left[ \left( \frac{\hat{Z}_{1,K} - Z}{Z} \right)^2 \right] + \nabla_{\theta,\phi} \mathbb{E} [R_2(\hat{Z}_{1,K})] + \nabla_{\theta,\phi} \log Z \\ &= -\frac{1}{2} \nabla_{\theta,\phi} \left( \frac{\text{Var}[\hat{Z}_{1,K}]}{Z^2} \right) + \nabla_{\theta,\phi} \mathbb{E} [R_2(\hat{Z}_{1,K})] + \nabla_{\theta,\phi} \log Z \\ &= -\frac{1}{2K} \nabla_{\theta,\phi} \left( \frac{\text{Var}[w_{1,1}]}{Z^2} \right) + \nabla_{\theta,\phi} \mathbb{E} [R_2(\hat{Z}_{1,K})] + \nabla_{\theta,\phi} \log Z. \end{aligned} \quad (\text{A.4})$$

Using a similar process as in variance case, it is now straightforward to show that  $\nabla_{\theta,\phi} \mathbb{E} [R_2(\hat{Z}_{1,K})] = O(1/K^2)$ , which is thus similarly dominated (also giving us (7)).

Finally, by combining (A.3) and (A.4) and noting that  $\sqrt{\frac{A}{K} + \frac{B}{K^2}} = \frac{A}{\sqrt{K}} + \frac{B}{2AK^{3/2}} + O\left(\frac{1}{K^{5/2}}\right)$  we have

$$\text{SNR}_{M,K}(\theta) = \left| \frac{\nabla_{\theta} \log Z - \frac{1}{2K} \nabla_{\theta} \left( \frac{\text{Var}[w_{1,1}]}{Z^2} \right) + O\left(\frac{1}{K^2}\right)}{\sqrt{\frac{1}{MKZ^4} \mathbb{E}[(Z \nabla_{\theta} w_{1,1} - w_{1,1} \nabla_{\theta} Z)^2] + \frac{1}{M} O\left(\frac{1}{K^2}\right)}} \right| \quad (\text{A.5})$$

$$= \sqrt{M} \left| \frac{Z^2 \sqrt{K} \left( \nabla_{\theta} \log Z - \frac{1}{2K} \nabla_{\theta} \left( \frac{\text{Var}[w_{1,1}]}{Z^2} \right) \right) + O\left(\frac{1}{K^{3/2}}\right)}{\sqrt{\mathbb{E}[(Z \nabla_{\theta} w_{1,1} - w_{1,1} \nabla_{\theta} Z)^2] + O\left(\frac{1}{K}\right)}} \right| \quad (\text{A.6})$$

$$= \sqrt{M} \left| \frac{\sqrt{K} \nabla_{\theta} Z - \frac{1}{2Z\sqrt{K}} \nabla_{\theta} \left( \frac{\text{Var}[w_{1,1}]}{Z^2} \right) + O\left(\frac{1}{K^{3/2}}\right)}{\sqrt{\mathbb{E}[w_{1,1}^2 (\nabla_{\theta} \log w_{1,1} - \nabla_{\theta} \log Z)^2] + O\left(\frac{1}{K}\right)}} \right| = O\left(\sqrt{MK}\right). \quad (\text{A.7})$$

For  $\phi$ , then because  $\nabla_{\phi} Z = 0$ , we instead have

$$\text{SNR}_{M,K}(\phi) = \sqrt{M} \left| \frac{\nabla_{\phi} \text{Var}[w_{1,1}] + O\left(\frac{1}{K}\right)}{2Z\sqrt{K} \sigma[\nabla_{\phi} w_{1,1}] + O\left(\frac{1}{\sqrt{K}}\right)} \right| = O\left(\sqrt{\frac{M}{K}}\right) \quad (\text{A.8})$$

and we are done.  $\square$

## B Derivation of Optimal Parameters for Gaussian Experiment

To derive the optimal parameters for the Gaussian experiment we first note that

$$\mathcal{J}(\theta, \phi) = \frac{1}{N} \log \prod_{n=1}^N p_\theta(x^{(n)}) - \frac{1}{N} \sum_{n=1}^N \text{KL} \left( Q_\phi(z_{1:K}|x^{(n)}) \parallel P_\theta(z_{1:K}|x^{(n)}) \right) \quad \text{where}$$

$$P_\theta(z_{1:K}|x^{(n)}) = \frac{1}{K} \sum_{k=1}^K q_\phi(z_1|x^{(n)}) \dots q_\phi(z_{k-1}|x^{(n)}) p_\theta(z_k|x^{(n)}) q_\phi(z_{k+1}|x^{(n)}) \dots q_\phi(z_K|x^{(n)}),$$

$Q_\phi(z_{1:K}|x^{(n)})$  is as per (2) and the form of the Kullback-Leibler (KL) is taken from (Le et al., 2018). Next, we note that  $\phi$  only controls the mean of the proposal so, while it is not possible to drive the KL to zero, it will be minimized for any particular  $\theta$  when the means of  $q_\phi(z|x^{(n)})$  and  $p_\theta(z|x^{(n)})$  are the same. Furthermore, the corresponding minimum possible value of the KL is independent of  $\theta$  and so we can calculate the optimum pair  $(\theta^*, \phi^*)$  by first optimizing for  $\theta$  and then choosing the matching  $\phi$ . The optimal  $\theta$  maximizes  $\log \prod_{n=1}^N p_\theta(x^{(n)})$ , giving  $\theta^* := \mu^* = \frac{1}{N} \sum_{n=1}^N x^{(n)}$ . As we straightforwardly have  $p_\theta(z|x^{(n)}) = \mathcal{N}(z; (x^{(n)} + \mu)/2, I/2)$ , the KL is then minimized when  $A = I/2$  and  $b = \mu/2$ , giving  $\phi^* := (A^*, b^*)$ , where  $A^* = I/2$  and  $b^* = \mu^*/2$ .

## C Additional Empirical Analysis of SNR

### C.1 Histograms for VAE

To complete the picture for the effect of  $M$  and  $K$  on the distribution of the gradients, we generated histograms for the  $K = 1$  (i.e. variational auto-encoder (VAE)) gradients as  $M$  is varied. As shown in Figure C.1a, we see the expected effect from the law of large numbers that the variance of the estimates decreases with  $M$ , but not the expected value.

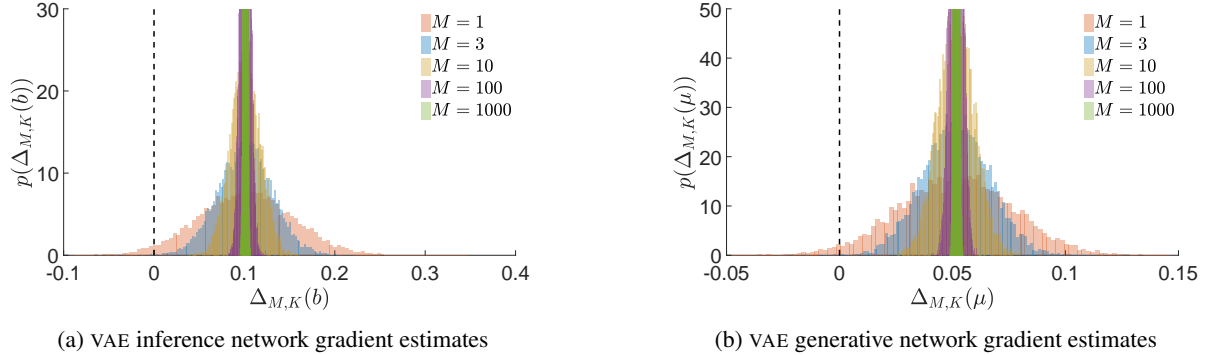

Figure C.1: Histograms of gradient estimates  $\Delta_{M,K}$  for the generative network and the inference network using the VAE ( $K = 1$ ) objectives with different values of  $M$ .

### C.2 Convergence of RMSE for Generative Network

As explained in the main paper, the SNR is not an entirely appropriate metric for the generative network – a low SNR is still highly problematic, but a high SNR does not indicate good performance. It is thus perhaps better to measure the quality of the gradient estimates for the generative network by looking at the root mean squared error (RMSE) to  $\nabla_\mu \log Z$ , i.e.  $\sqrt{\mathbb{E} [\|\Delta_{M,K} - \nabla_\mu \log Z\|_2^2]}$ . The convergence of this RMSE is shown in Figure C.2 where the solid lines are the RMSE estimates using  $10^4$  runs and the shaded regions show the interquartile range of the individual estimates. We see that increasing  $M$  in the VAE reduces the variance of the estimates but has negligible effect on the RMSE due to the fixed bias. On the other hand, we see that increasing  $K$  leads to a monotonic improvement, initially improving at a rate  $O(1/K)$  (because the bias is the dominating term in this region), before settling to the standard Monte Carlo convergence rate of  $O(1/\sqrt{K})$  (shown by the dashed lines).

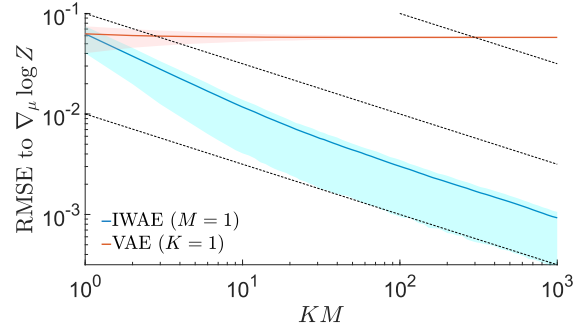

Figure C.2: RMSE in  $\mu$  gradient estimate to  $\nabla_\mu \log Z$

### C.3 Experimental Results for High Variance Regime

We now present empirical results for a case where our weights are higher variance. Instead of choosing a point close to the optimum by offsetting parameters with a standard deviation of 0.01, we instead offset using a standard deviation of 0.5. We further increased the proposal covariance to  $I$  to make it more diffuse. This is now a scenario where the model is far from its optimum and the proposal is a very poor match for the model, giving very high variance weights.

We see that the behavior is the same for variation in  $M$ , but somewhat distinct for variation in  $K$ . In particular, the signal-to-noise ratio (SNR) and DSNR only decrease slowly with  $K$  for the inference network, while increasing  $K$  no longer has much benefit for the SNR of the inference network. It is clear that, for this setup, the problem is very far from the asymptotic regime in  $K$  such that our theoretical results no longer directly apply. Nonetheless, the high-level effect observed is still that the SNR of the inference network deteriorates, albeit slowly, as  $K$  increases.

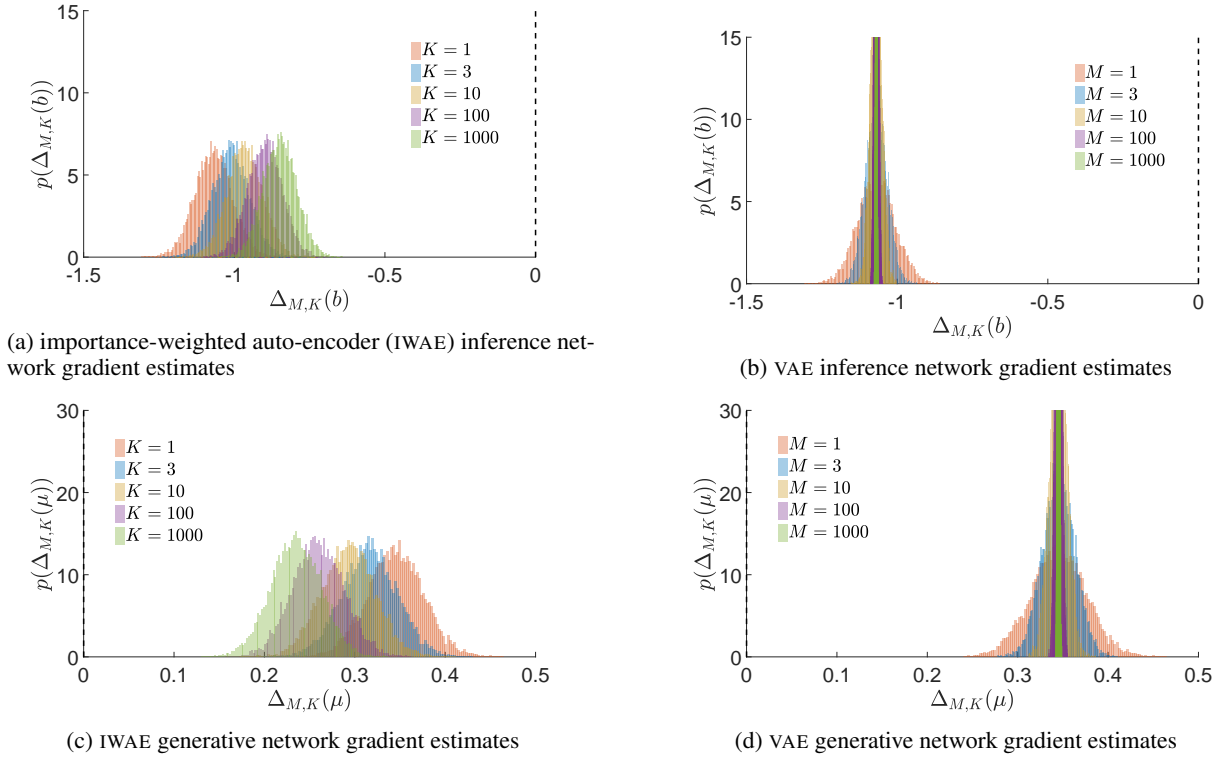

Figure C.3: Histograms of gradient estimates as per Figure 1.

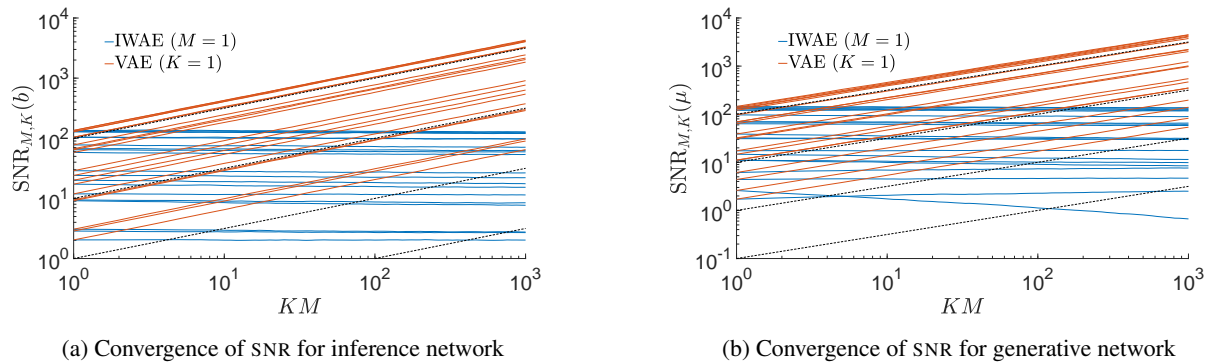

Figure C.4: Convergence of signal-to-noise ratios of gradient estimates as per Figure 2.

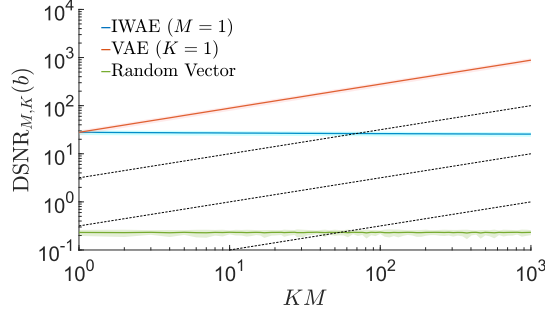

(a) Convergence of DSNR for inference network

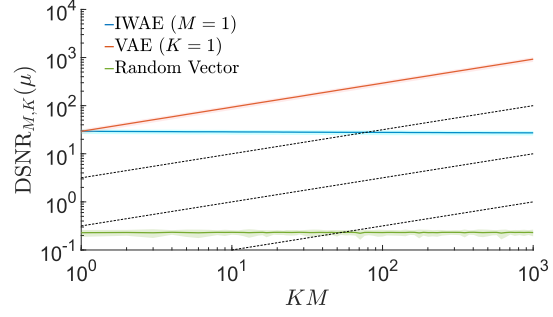

(b) Convergence of DSNR for generative network

Figure C.5: Convergence of directional signal-to-noise ratio of gradients estimates as per Figure 3.

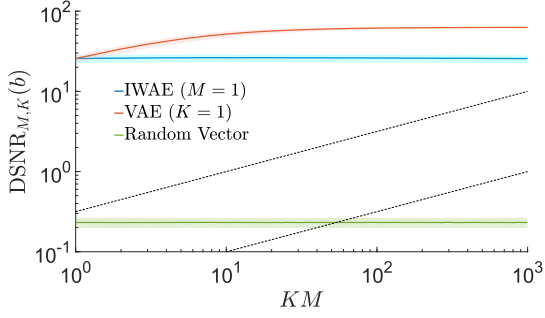

(a) Convergence of DSNR for inference network

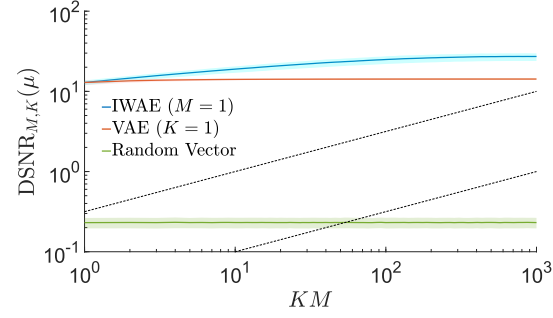

(b) Convergence of DSNR for generative network

 Figure C.6: Convergence of directional signal-to-noise ratio of gradient estimates where the true gradient is taken as  $\mathbb{E}[\Delta_{1,1000}]$  as per Figure 4.

## D Convergence of Deep Generative Model for Alternative Parameter Settings

Figure D.1 shows the convergence of the introduced algorithms under different settings to those shown in Figure 5. Namely we consider  $M = 4, K = 16$  for partially importance-weighted auto-encoder (PIWAE) and multiply importance-weighted auto-encoder (MIWAE) and  $\beta = 0.05$  for combination importance-weighted auto-encoder (CIWAE). These settings all represent tighter bounds than those of the main paper. Similar behavior is seen in terms of the IWAE-64 metric for all algorithms. PIWAE produced similar mean behavior for all metrics, though the variance was noticeably increased for  $\log \hat{p}(x)$ . For CIWAE and MIWAE, we see that the parameter settings represent an explicit trade-off between the generative network and the inference network:  $\log \hat{p}(x)$  was noticeably increased for both, matching that of IWAE, while  $-\text{KL}(Q_\phi(z|x)||P_\theta(z|x))$  was reduced. Critically, we see here that, as observed for PIWAE in the main paper, MIWAE and CIWAE are able to match the generative model performance of IWAE whilst improving the KL metric, indicating that they have learned better inference networks.

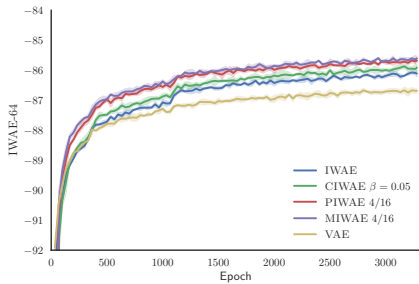
 (a) IWAE<sub>64</sub>
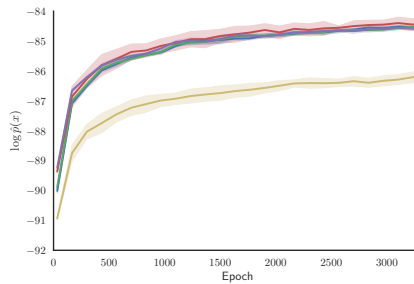
 (b)  $\log \hat{p}(x)$ 
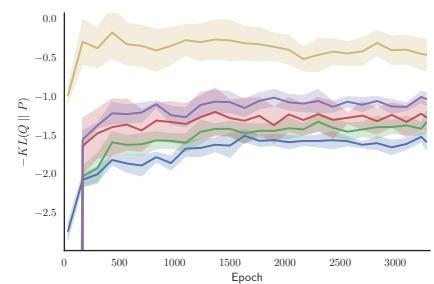
 (c)  $-\text{KL}(Q_\phi(z|x)||P_\theta(z|x))$ 

Figure D.1: Convergence of different evaluation metrics for each method. Plotting conventions as per Figure 5.

## E Convergence of Toy Gaussian Problem

We finish by assessing the effect of the outlined changes in the quality of the gradient estimates on the final optimization for our toy Gaussian problem. Figure E.1 shows the convergence of running Adam (Kingma & Ba, 2014) to optimize  $\mu$ ,  $A$ , and  $b$ . This suggests that the effects observed predominantly transfer to the overall optimization problem. Interestingly, setting  $K = 1$  and  $M = 1000$  gave the best performance on learning not only the inference network parameters, but also the generative network parameters.

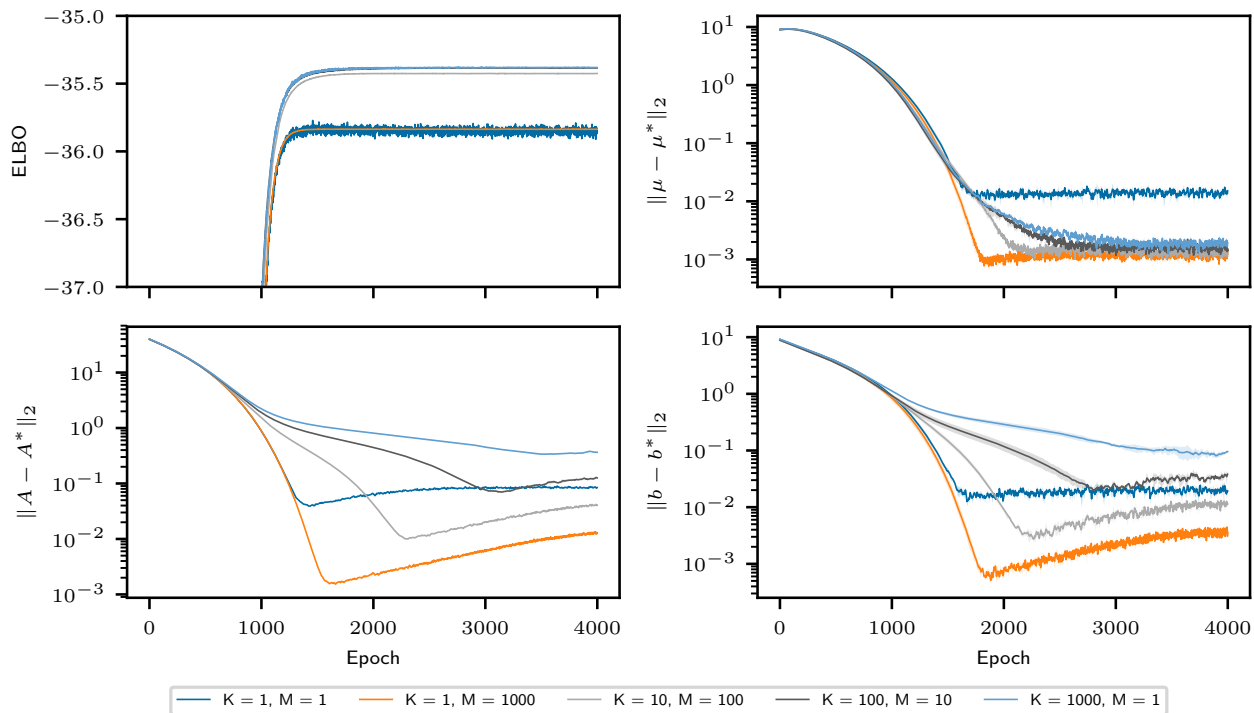

Figure E.1: Convergence of optimization for different values of  $K$  and  $M$ . (Top, left)  $\text{ELBO}_{\text{IS}}$  during training (note this represents a different metric for different  $K$ ). (Top, right)  $L_2$  distance of the generative network parameters from the true maximizer. (Bottom)  $L_2$  distance of the inference network parameters from the true maximizer. Plots show means over 3 repeats with  $\pm 1$  standard deviation. Optimization is performed using the Adam algorithm with all parameters initialized by sampling from the uniform distribution on  $[1.5, 2.5]$ .

## References

- Fort, G., Gobet, E., and Moulines, E. Mcmc design-based non-parametric regression for rare event. application to nested risk computations. *Monte Carlo Methods and Applications*, 23(1):21–42, 2017.
- Hesterberg, T. C. *Advances in importance sampling*. PhD thesis, Stanford University, 1988.
- Kingma, D. and Ba, J. Adam: A method for stochastic optimization. *arXiv preprint arXiv:1412.6980*, 2014.
- Le, T. A., Igl, M., Rainforth, T., Jin, T., and Wood, F. Auto-encoding sequential Monte Carlo. In *ICLR*, 2018.
- Rainforth, T. *Automating Inference, Learning, and Design using Probabilistic Programming*. PhD thesis, 2017.
- Rainforth, T., Cornish, R., Yang, H., Warrington, A., and Wood, F. On nesting Monte Carlo estimators. In *ICML*, 2018.
